# Supplementary material for: Binding Sites for Luminescent Amyloid Biomarkers from non-Biased Molecular Dynamics Simulations
Source: arXiv:1808.07552 ancillary file (2018-08-22)
Supplement: Supplementary file 1 [file supplement.pdf]

# Supplementary Material to Binding Sites for Luminescent Amyloid Biomarkers from non-Biased Molecular Dynamics Simulations

Carolin König,† Robin Skånberg,‡ Ingrid Hotz,‡ Anders Ynnerman,‡ Patrick Norman,† and Mathieu Linares*,†,¶

†*School of Biotechnology, Division of Theoretical Chemistry & Biology, KTH Royal Institute of Technology, Roslagstullsbacken 15, 114 21 Stockholm, Sweden*

‡*Linköpings University, Department for Media and Information Technology, Norrköping, Sweden*

¶*Swedish e-Science Research Centre (SeRC), KTH Royal Institute of Technology, 104 50 Stockholm, Sweden*

E-mail: linares@kth.se

## Computational details

For all molecular dynamics (MD) simulations, we employed the Gromacs program package[1–3] in combination with the CHARMM27 force field[4–6] for the protein and TIP3P[7] for the water solvent. The forcefield for the oligo-thiophene chromophore was taken from Ref. 8. In all simulations, we used periodic boundary conditions. The MD simulations in an $NPT$ ensemble were carried out maintaining the temperature at 300 K with the v-Rescale

thermostat and coupling constant of 0.2 ps. A Berendsen barostat with a coupling contant of 1 ps was employed to maintain the pressure at 1 atm. In case of th full periodic model (see below), we used a semi-isotropic berendsen barostat only in the two directions perpendicular to the axis of the amyloid fibril. The electrostatic and van der Waals interactions where both calculated with a cut-off distance of 1.5 nm. Subsequently, we propagated the system in an $NVT$ ensemble. This procedure of $NPT$ and then $NVT$ ensemble simulation has been performed for all models. If not stated otherwise, we kept all internal degrees freedom of the water molecules as well as all bonds constrained during the MD simulations. For the exact simulation times, we refer to the description of the model setup.

The time-dependent density functional (TDDFT) calculations were performed with the Gaussian program package[9] in combination with the CAM-B3LYP functional[10] and the 6-31+G(d)[11,12] basis set. We have calculated the lowest 20 excitations.

# Model setup

## Full periodic model for the amyloid fibril

The model setup is based on the PDB entry 5OQV.[13] For this, we cut out chain A of this protein model and repeatedly produced copies of it by an rotation operation by 179.29 degrees around the middle z axis of this bundle followed by a translation of 2.485 Å exploiting the approximate $2_1$ screw symmetry reported in Ref. 13. The applied rotatation angle and displacements have been estimated from the structure provided in 5OQV. The displacement has been chosen 0.15 Å larger than this estimate to account for the expansion of the protein at room temperature compared to the cryo-EM conditions. With 253 copies of chain A in this way we generated a half turn of the complete helix and can, due to the symmetry, employ perioidic boundary conditions for the helix. The simulation box in that dimension amounts to about 63 nm. For the other two dimensions, we set the dimension of the simulation box to 22 nm and added water solvent. Additionally, 759 sodium ions were added to obtain an

overall neutral simulation box. With this model we performed a molecular dynamics with semi-isotropic barostat. Keeping only the internal modes of the water molecules constrained, we obtain a box dimension of 64.5 nm along the main axis and 21.7 nm in the perpendicular dimensions.

## Full periodic model for the amyloid fibril with p-FTAA molecules

The full periodic model for the amyloid fibril with p-FTAA molecules was constructed from the final structure of the above-described full periodic model of the amyloid fibril. We added 100 p-FTAA molecules to the system, neutralized it accordingly with sodium atoms, and repeated the $NPT$ equilibration for 1.5 ns without bond constraints apart from the water molecules. This lead a simulation box dimension of 64.3 nm along the main axis and 21.6 nm in the perpendicular dimensions, i.e., to very similar box dimension as without the LCO molecules.

Program constraints in Gromacs allowed us to monitor the interaction of only 61 biomarker molecules with the protein (64 energy groups in total: 61 molecules, protein, solvent, rest of the system). For this reason, we first performed an $NVT$ ensemble simulation for 16.8 ns and then selected those 61 chromophores that are close to the amyloid fibril for the analysis in the remaining part of the total $NVT$ simulation time of 40 ns. We report only on the results for these tracked molecules in the main text. A snapshot after 16.8 ns is shown in Figure S-1. We note that for all p-FTAA molecules that come in the proximity of the amyloid fibril during the whole simulation time of 40 ns, we monitor the interaction energies with the protein.

## Smaller binding site model

To generate the smaller binding site model, we used our large model after 16.8 ns simulation time and cut out the surroundings of the tightest bound p-FTAA molecule (termed p-FTAA*). The included protein consists of eleven protein chains at the side where the

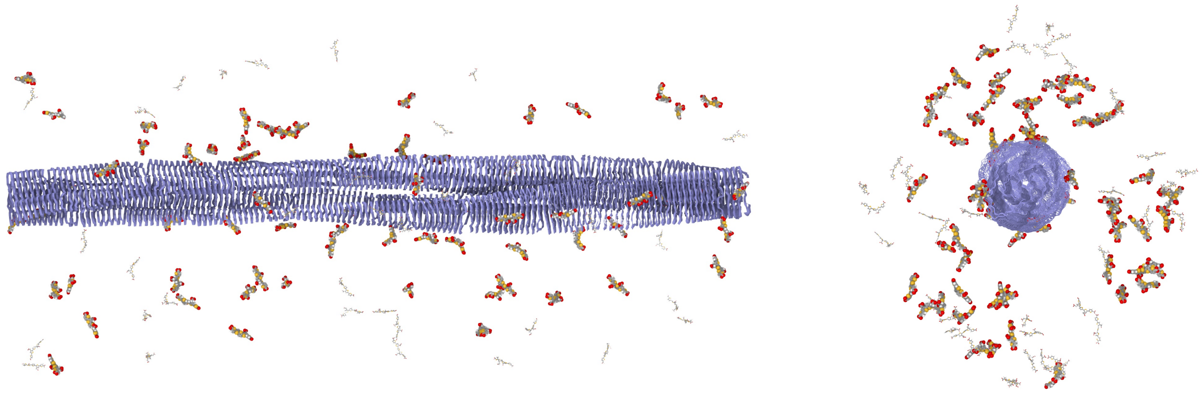

Figure S-1: Simulation snapshot after 16.8 ns. Left: side view. Right: front view. The monitored p-FTAA molecules are shown in red and the non-monitored ones in grey.

p-FTAA* molecule is attached and ten on the other side (see Figure S-2). We have created

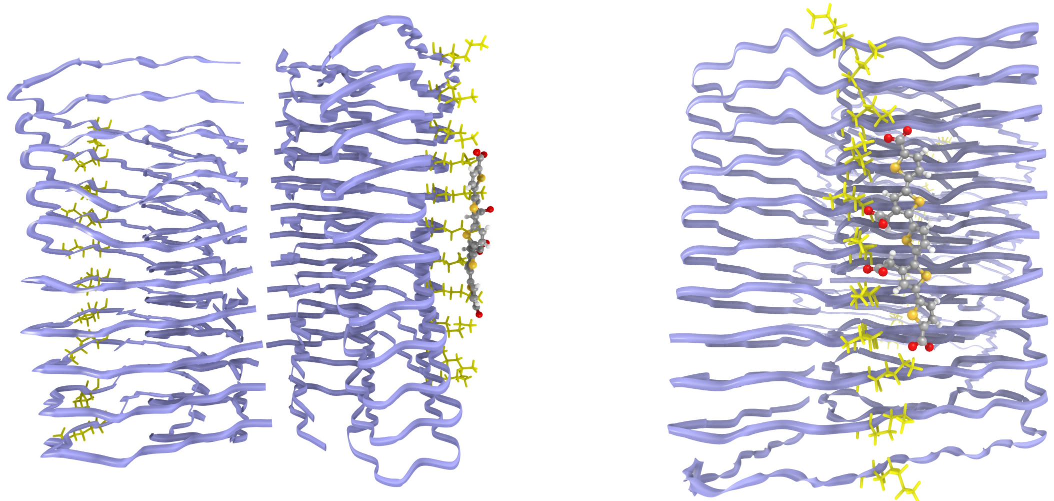

Figure S-2: Small model for the p-FTAA* molecule at a small part of the amyloid fibril. The fibril is shown in blue, the lysine 16 side chains in yellow. Left: side view. Right: front view.

a water solvation box around this model of the size 15 nm $\times$ 15 nm $\times$ 18 nm, where the latter is the axis of the amyloid fibril segment, and neutralized the box by adding sodium ions. For this model, we have performed with 13.8 ns $NPT$ ensemble simulations and subsequently an $NVT$ ensemble simulation for 62.4 ns. All molecular dynamics settings where chosen analogously to the one for the full system. One difference is that in this case the we employed a Berendsen barostat in all directions. Moreover, in for this reduced model, the

outer-most protein chains are kept constrained to their positions. All data reported is taking from the $NVT$ simulations.

## p-FTAA in water

For the p-FTAA-in-water case, we solvated one p-FTAA molecule in a 5 nm $\times$ 5 nm $\times$ 5 nm water box with a density of 1 $\frac{g}{cm^3}$ and performed an $NVT$ ensemble simulation for 100 ns with the almost identical settings as for the other models. The only difference is that, in this case, we did not constrain the bonds within the p-FTAA molecule during $NVT$ simulation. From this trajectory, we extracted 1001 snapshots, replaced the carboxy groups by hydrogen atoms and performed the TDDFT calculation in vacuum.

## Example for an approaching trajectory

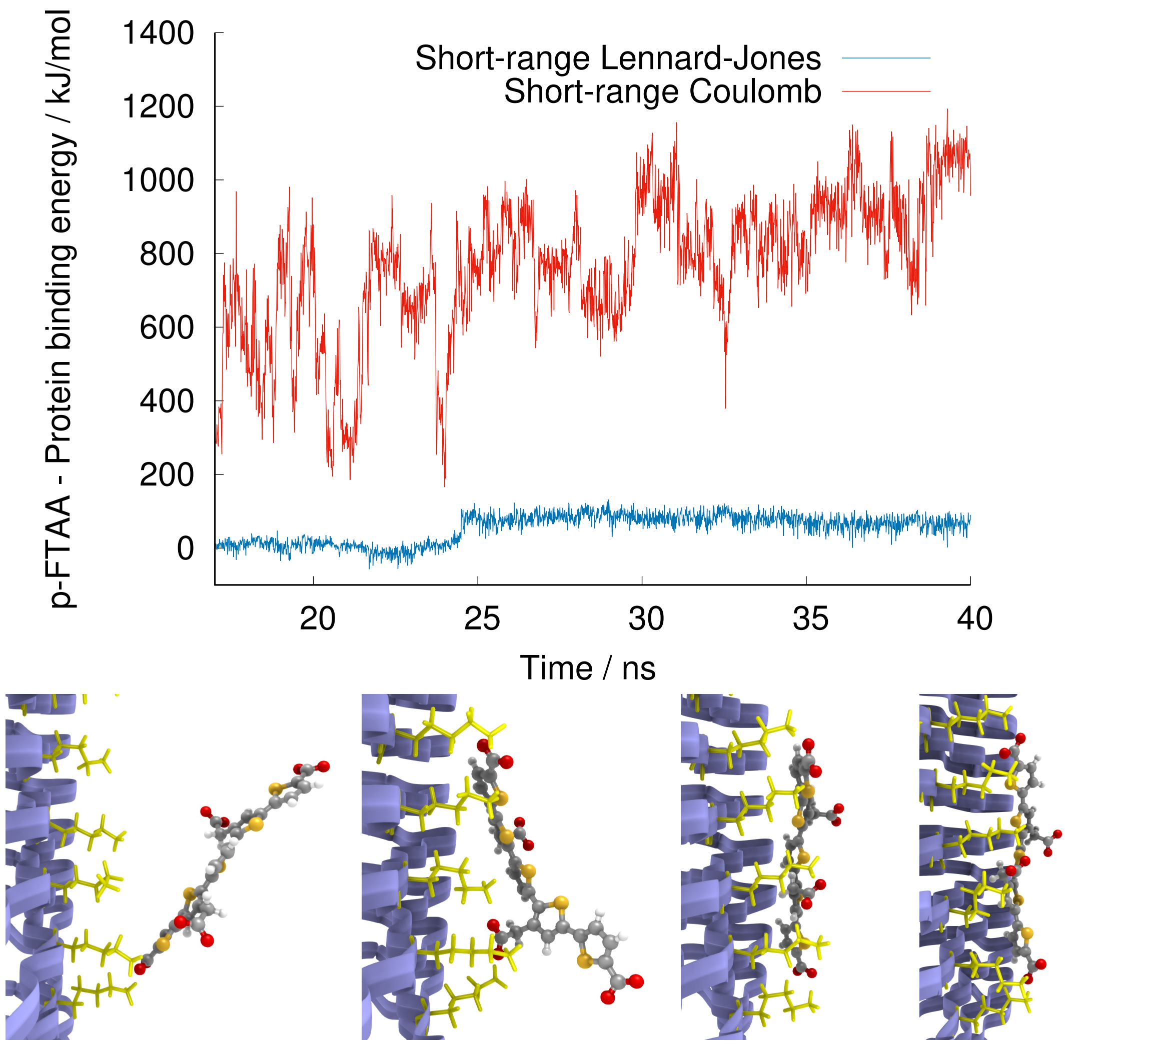


Figure S-3: Example for approaching characteristics at of one p-FTAA molecule at the amyloid protein. Top figure: Short-range Lennard–Jones and Coulomb binding energies. Bottom figures: Snap-shots at 16.8 ns, 24.3 ns, 24.6 ns, and 40.0 ns, showing that the clear increase of the in Lennard–Jones binding energy at about 24.5 ns is accompanied with lying down of the probe on the protein surface.

## Planarity–Absorption energy plots for an LCO in water

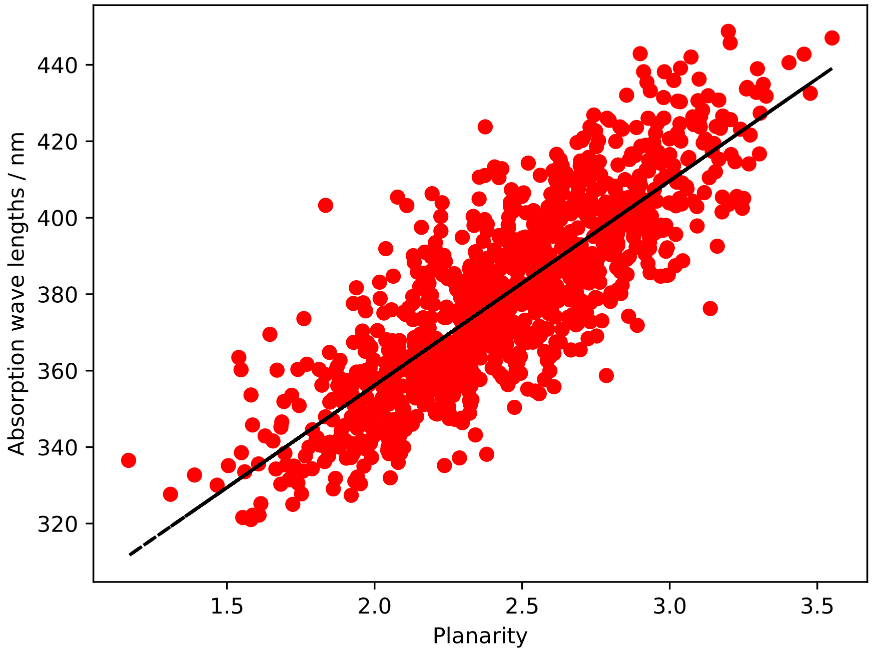


Figure S-4: Calculated first absorption energy of p-FTA for 1001 conformations from a converged molecular dynamics simulation in water. Linear regression yields $\Delta E(p)[\mathrm{nm}] = 53.48\ \mathrm{nm} \times p + 249.21\ \mathrm{nm}$, where $p$ is the planarity and $R^2 = 0.68$.

## Visualization

The analysis of the binding mode of p-FTAA on the amyloid fibril as been made with VAMD, a new visualization environment tailored for exploration of molecular dynamics simulations. VAMD incorporates linked interactive 3D exploration of geometry and statistical analysis using dynamic temporal windowing and animation. It also exposes filters for chosen simulation properties and data, which enables the ability to explore the data and find spatial, temporal and statistical patterns.

# References

(1) Berendsen, H.; van der Spoel, D.; van Drunen, R. GROMACS: A message-passing parallel molecular dynamics implementation. *Comput. Phys. Commun.* **1995**, *91*, 43–56.

(2) Lindahl, E.; Hess, B.; van der Spoel, D. GROMACS 3.0: a package for molecular simulation and trajectory analysis. *J. Mol. Model.* **2001**, *7*, 306–317.

(3) Van Der Spoel, D.; Lindahl, E.; Hess, B.; Groenhof, G.; Mark, A. E.; Berendsen, H. J. C. GROMACS: Fast, flexible, and free. *J. Comput. Chem.* **2005**, *26*, 1701–1718.

(4) Brooks, B. R.; Bruccoleri, R. E.; Olafson, B. D.; States, D. J.; Swaminathan, S.; Karplus, M. CHARMM: A program for macromolecular energy, minimization, and dynamics calculations. *J. Comput. Chem.* **1983**, *4*, 187–217.

(5) Brooks, B. R. et al. CHARMM: The biomolecular simulation program. *J. Comput. Chem.* **2009**, *30*, 1545–1614.

(6) Bjelkmar, P.; Larsson, P.; Cuendet, M. A.; Hess, B.; Lindahl, E. Implementation of the CHARMM Force Field in GROMACS: Analysis of Protein Stability Effects from Correction Maps, Virtual Interaction Sites, and Water Models. *J. Chem. Theory Comput.* **2010**, *6*, 459–466.

(7) Jorgensen, W. L.; Chandrasekhar, J.; Madura, J. D.; Impey, R. W.; Klein, M. L. Comparison of simple potential functions for simulating liquid water. *J. Chem. Phys.* **1983**, *79*, 926–935.

(8) Sjöqvist, J.; Linares, M.; Mikkelsen, K. V.; Norman, P. QM/MM-MD Simulations of Conjugated Polyelectrolytes: A Study of Luminescent Conjugated Oligothiophenes for Use as Biophysical Probes. *J. Phys. Chem. A* **2014**, *118*, 3419–3428.

(9) Frisch, M. J. et al. Gaussian 09. 2016.

(10) Yanai, T.; Tew, D. P.; Handy, N. C. A new hybrid exchange-correlation functional using the Coulomb-attenuating method (CAM-B3LYP). *Chem. Phys. Lett.* **2004**, *393*, 51–57.

(11) Petersson, G. A.; Bennett, A.; Tensfeldt, T. G.; Al-Laham, M. A.; Shirley, W. A.; Mantzaris, J. A complete basis set model chemistry. I. The total energies of closed-shell atoms and hydrides of the first-row elements. *J. Chem. Phys.* **1988**, *89*, 2193–2218.

(12) Petersson, G. A.; Al-Laham, M. A. A complete basis set model chemistry. II. Open-shell systems and the total energies of the first-row atoms. *J. Chem. Phys.* **1991**, *94*, 6081–6090.

(13) Gremer, L.; Schölzel, D.; Schenk, C.; Reinartz, E.; Labahn, J.; Ravelli, R. B. G.; Tusche, M.; Lopez-Iglesias, C.; Hoyer, W.; Heise, H.; Willbold, D.; Schröder, G. F. Fibril structure of amyloid-$\beta$(1-42) by cryo-electron microscopy. *Science* **2017**, *358*, 116–119.
